# Supplementary material for: Two-loop QED corrections to the scattering of four massive leptons
Source: arXiv:2311.06385 ancillary file (2023-11-10)
Supplement: Supplementary file 1 [file README.pdf]

# Ancillary Files for “Two-loop QED corrections to the scattering of four massive leptons”

Maximilian Delto,<sup>1,\*</sup> Claude Duhr,<sup>2,†</sup> Lorenzo Tancredi,<sup>1,‡</sup> and Yu Jiao Zhu<sup>2,§</sup>

<sup>1</sup>*Physik Department, James-Frank-Straße 1, Technische Universität München,  
D-85748 Garching, Germany*

<sup>2</sup>*Bethe Center for Theoretical Physics, Universität Bonn, D-53115, Germany*

In this note we explain the definitions and conventions for the ancillary files associated with the arXiv submission of “Two-loop QED corrections to the scattering of four massive leptons”.

## KINEMATICS AND MASS-EXPANSION

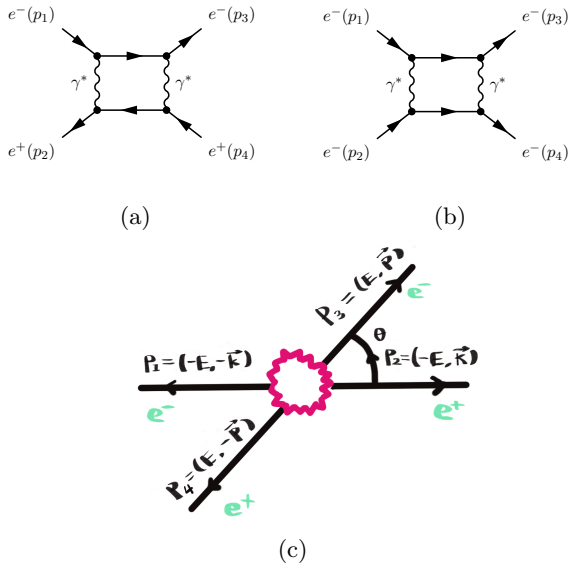

FIG. 1: One-loop diagram (a) for Bhabha scattering:  $e^-(p_1)e^+(p_2) \rightarrow e^-(p_3)e^+(p_4)$  and diagram (b) for Møller scattering:  $e^-(p_1)e^-(p_2) \rightarrow e^-(p_3)e^-(p_4)$ . External momenta are out-going and on-shell:  $p_1 + p_2 + p_3 + p_4 = 0, p_i^2 = m^2$ .

The kinematics are illustrate in fig. (??) , where the Mandelstam variables are defined as

$$s = (p_1 + p_2)^2, \quad t = (p_1 + p_3)^2, \quad u = (p_2 + p_3)^2 \quad (1)$$

with  $s + t + u = 4m^2$ . In terms of the scattering angle and the center of mass energy, we have

$$s = 4E^2 = E_{\text{CM}}^2, \quad t = 2m^2 - 2E^2 + 2\vec{k} \cdot \vec{p}, \quad (2)$$

and

$$|\vec{k}| = |\vec{p}| = \sqrt{E^2 - m^2}, \quad \vec{k} \cdot \vec{p} = |\vec{k}| |\vec{p}| \cos \theta, \quad (3)$$

moreover,

$$-t/s = (1 - m^2/E^2) \sin^2(\theta/2). \quad (4)$$

We also introduce the following set of variables for the mass expansion,

$$-t/s \equiv \frac{1}{2} - \frac{1}{4y_p} - \frac{y_p}{4}, \quad \frac{m^2}{s} \equiv x^2. \quad (5)$$

Let  $y_p = e^{i\eta}$ , then  $-t/s = \sin^2(\eta/2)$ , so in the high-energy limit

$$\eta \approx \theta, \quad \text{and} \quad x = m/E_{\text{CM}}. \quad (6)$$

We use  $x$  – the ratio between the electron mass and the center-of-mass energy as our mass-expansion parameter;  $y_p$  will be the function argument of Harmonic Polylogarithms (HPLs). Since  $-t/s$  as function of  $\eta$  is invariant under inversion  $\eta \rightarrow -\eta$ , we assume  $0 < \eta < \pi$ . We emphasize that formulas are only valid in this domain.

## PERTURBATIVE EXPANSION AND SUM OF SPINS

We first describe our choice for the renormalization schemes. While the wave function renormalizations are always performed in on-shell (OS) scheme, the redefinition of the bare coupling constant is however performed separately in two UV renormalization schemes with  $r \in \{\overline{\text{MS}}, \text{OS}\}$ . The running coupling constant is given by  $a_e = \frac{\alpha_e(\mu)}{4\pi}$  in  $\overline{\text{MS}}$  scheme, and the physical on-shell coupling is given by  $a_e = a = \frac{\alpha}{4\pi}$  in the OS scheme. Note that they are related through

$$\alpha_e(\mu) = \alpha \left[ 1 + \frac{4}{3} \frac{\alpha}{4\pi} \ln \frac{\mu^2}{m^2} + \mathcal{O} \left( \frac{\alpha}{4\pi} \right)^2 \right]. \quad (7)$$

In addition to the dependence on UV renormalization schemes, the amplitudes are further dimensional regularization scheme-dependent quantities. We work in ‘t Hooft-Veltman (tHV) dimensional regularization scheme and decompose the scattering amplitude into eight independent Lorentz-covariant, physical tensors  $T_i$ , given as in eq. (6) of our manuscript. To perform the sum and averaging of the initial and final state spins, one resorts to the unpolarized spin correlation functions in `spin_unpol-correlation.m`.

As analytic functions, the amplitudes depend on the scale logarithm  $\ln(u2m2) = \ln(\mu^2/m^2)$ , the mass-expansion parameter  $x = m/E_{\text{CM}}$ , and the scattering angle  $\eta \approx \theta$ .

We then describe perturbative expansions of the results. For the UV-renormalized amplitudes of Bhabha  $e^-(p_1) + e^+(p_2) \rightarrow e^-(p_3) + e^+(p_4)$  and Møller  $e^-(p_1) + e^-(p_2) \rightarrow e^-(p_3) + e^-(p_4)$ , we have the following perturbative expansions in terms of the coupling constant

$$\mathcal{A}^r(\alpha_e, m, s, t, \epsilon) = 4\pi\alpha_e \sum_i a_e^i A[i] \left( \epsilon, \frac{\mu^2}{m^2}, x, \eta \right). \quad (8)$$

Similarly, for the finite remainder functions

$$\mathcal{C}^{\text{OS}}(\alpha, m, s, t) = 4\pi\alpha \sum_i a^i \text{wilsonC}[i] \left( \frac{\mu^2}{m^2}, x, \eta \right). \quad (9)$$

The various coefficients  $\text{wilsonC}[i]$  and  $A[i]$  are collected in file folder ‘Bhabha’ and ‘Moller’, these are respectively the results for Bhabha scattering and Møller scattering. Note that in the folder ‘Moller’ we have include mass-expansions thorough order  $x^{20}$  and exact results at 1-loop.

To be more explicit, the finite remainder functions are called

$$\text{wilsonC}[0,0], \quad \text{wilsonC}[1,0], \quad \text{wilsonC}[2,0], \quad (10)$$

and

$$\text{wilsonC}[0], \quad \text{wilsonC}[1], \quad \text{wilsonC}[2], \quad (11)$$

where  $\text{wilsonC}[i,j] = \sum_{\text{pol}} \text{wilsonC}[i] \times \text{wilsonC}^*[j]$  corresponds to the unpolarized contribution from  $\frac{1}{4}(4\pi\alpha)^2 \sum_{\text{pol}} a^{i+j} \text{wilsonC}[i] \times \text{wilsonC}^*[j]$ , and the factor  $\frac{1}{4}$  stands for averaging over initial states.

## LIST OF FILES

Interested readers can use `README.nb` and load the following files:

Results renormalized in OS scheme:

1. `A-pol-HV-OS.m`, the UV renormalized amplitude with on-shell charge.
2. `hardAmp-pol-OS.m` and `hardAmp-unpol-OS.m`, the finite remainder functions.

Results renormalized in OS- $\overline{\text{MS}}$  mixed scheme:

1. `A-pol-HV-aeMSb.m`, the UV renormalized amplitude with  $\overline{\text{MS}}$  charge.

---

\* maximilian.delto@tum.edu

† cduhr@uni-bonn.de

‡ lorenzo.tancredi@tum.de

§ yzhu@uni-bonn.de
